# Supplementary material for: Discrete gene replication events drive coupling between the cell cycle and circadian clocks
Source: arXiv:1510.05850 source file (2015-10-20)
Supplement: Supplementary file 1 [file Paijmans_Arxiv_SI.pdf]

,

# Supplementary information for "Discrete gene replication events drive coupling between the cell cycle and circadian clocks"

Joris Paijmans,[1] Mark Bosman,[1] Pieter Rein ten Wolde,[1] and David K. Lubensky[2]

[1] *FOM Institute AMOLF, Science Park 104, 1098 XG Amsterdam, The Netherlands*

[2] *Department of Physics, University of Michigan, Ann Arbor, MI 48109-1040*

## I. THE DETERMINISTIC NEGATIVE TRANSCRIPTIONAL FEEDBACK OSCILLATOR (FIGS. 2 AND 4)

Here we describe the negative transcriptional feedback oscillator (NTFO) studied in the main text, together with its parameters. The model consists of a single variable, $C(t)$, describing the concentration of proteins that inhibit their own production:

$$\frac{dC(t)}{dt} = \beta\,\tilde{G}(t)\,\frac{K_c^n}{K_c^n + C(t-\Delta)^n} - \mu_{\rm tot} C(t). \tag{S1}$$

We impose a fixed delay $\Delta$ between the initiation of transcription and the appearance of functional proteins. Therefore, protein production at time $t$ is proportional to the gene copy number $g(t-\Delta)$ at time $t-\Delta$. These proteins enter the cell volume $V(t)$ at time $t$. Combining these two effects, the protein synthesis rate per unit volume at time $t$ is thus proportional to the *protein production density* $\tilde{G}(t) \equiv g(t-\Delta)/V(t)$. Because the production at time $t$ depends on the state of the promoter at $t-\Delta$, the Hill function describing auto-regulation with Hill coefficient $n$ and concentration of half-maximal repression $K_c$, is evaluated with the delayed concentration $C(t-\Delta)$. Proteins are degraded with a total rate $\mu_{\rm tot} = \mu_{\rm d} + \mu_{\rm act}$, where $\mu_{\rm d}$ describes dilution due to cell growth, and $\mu_{\rm act}$ describes possible active degradation. Including both terms allows us to vary the doubling time $T_{\rm d}$ while holding $\mu_{\rm tot}$ constant and hence to distinguish the trivial influence of the cell cycle on the clock through the dilution rate $\mu_{\rm d}$ from other effects. This model is a deterministic one, based on mean-field chemical rate equations. A stochastic version that takes into account the intrinsic stochasticity of biochemical reactions is introduced further below.

Parameters used in the simulations are: $\beta = 6.0 \cdot 10^3 {\rm h}^{-1}$; $K_c = 1.0\mu$M; $n = 2$; $\mu_{\rm tot} = 0.2{\rm h}^{-1}$; $\Delta = 8$h. Details regarding the simulations are given in the Methods section of this document. The principal results of this model are presented in Figs. 2 and 4 of the main text.

## II. ZWICKER TTC-PPC MODEL (FIGS. 4 AND 5)

The PPC-TTC model of Zwicker *et al.* consists of a protein phosphorylation cycle (PPC) combined with a transcription-translation cycle (TTC) [35]. The PPC model is based on that of Van Zon *et al.* [25]. In this model, each KaiC hexamer has an intrinsic tendency to progress through a phosphorylation cycle, while the phosphorylation cycles of the individual hexamers are synchronized via the mechanism of differential affinity: KaiA stimulates KaiC phosphorylation, but the limited supply of KaiA binds preferentially to those KaiC hexamers that are falling behind in the cycle, forcing the front runners to slow down and allowing the laggards to catch up. The model includes the following reactions [25]:

$$\mathrm{C}_i \underset{b_i}{\overset{f_i}{\rightleftarrows}} \widetilde{\mathrm{C}}_i, \qquad \mathrm{C}_i + \mathrm{A} \underset{k_i^{\rm Ab}}{\overset{k_i^{\rm Af}}{\rightleftarrows}} \mathrm{AC}_i \overset{k_{\rm pf}}{\rightarrow} \mathrm{C}_{i+1} + \mathrm{A}, \tag{S2}$$

$$\widetilde{\mathrm{C}}_i + \mathrm{B} \underset{\tilde{k}_i^{\rm Bb}}{\overset{2\tilde{k}_i^{\rm Bf}}{\rightleftarrows}} \mathrm{B}\widetilde{\mathrm{C}}_i, \qquad \mathrm{B}\widetilde{\mathrm{C}}_i + \mathrm{B} \underset{2\tilde{k}_i^{\rm Bb}}{\overset{\tilde{k}_i^{\rm Bf}}{\rightleftarrows}} \mathrm{B}_2\widetilde{\mathrm{C}}_i, \tag{S3}$$

$$\mathrm{B}_x\widetilde{\mathrm{C}}_i + \mathrm{A} \underset{\tilde{k}_i^{\rm Ab}}{\overset{x\tilde{k}_i^{\rm Af}}{\rightleftarrows}} \mathrm{AB}_x\widetilde{\mathrm{C}}_i, \qquad \mathrm{AB}_2\widetilde{\mathrm{C}}_i + \mathrm{A} \underset{2\tilde{k}_i^{\rm Ab}}{\overset{\tilde{k}_i^{\rm Af}}{\rightleftarrows}} \mathrm{A}_2\mathrm{B}_2\widetilde{\mathrm{C}}_i, \tag{S4}$$

$$\mathrm{C}_i \underset{k_{\rm dps}}{\overset{k_{\rm ps}}{\rightleftarrows}} \mathrm{C}_{i+1}, \qquad \widetilde{\mathrm{C}}_i \underset{\tilde{k}_{\rm dps}}{\overset{\tilde{k}_{\rm ps}}{\rightleftarrows}} \widetilde{\mathrm{C}}_{i+1}, \tag{S5}$$

$$\mathrm{B}_x\widetilde{\mathrm{C}}_i \underset{\tilde{k}_{\rm dps}}{\overset{\tilde{k}_{\rm ps}}{\rightleftarrows}} \mathrm{B}_x\widetilde{\mathrm{C}}_{i+1}, \qquad \mathrm{A}_y\mathrm{B}_x\widetilde{\mathrm{C}}_i \underset{\tilde{k}_{\rm dps}}{\overset{\tilde{k}_{\rm ps}}{\rightleftarrows}} \mathrm{A}_y\mathrm{B}_x\widetilde{\mathrm{C}}_{i+1}\;. \tag{S6}$$

Here, $\mathrm{C}_i$ denotes a KaiC hexamer in the active conformational state, in which the number $i$ of phosphorylated monomers tends to increase, and $\widetilde{\mathrm{C}}_i$ denotes a KaiC hexamer in the inactive conformational state in which $i$ tends to decrease; A denotes a KaiA dimer, and B denotes a KaiB dimer. The reactions $\mathrm{C}_i \rightleftarrows \widetilde{\mathrm{C}}_i$ in Eq. S2 model the conformational transitions between active and inactive KaiC; the second set of reactions in Eq. S2 describe phosphorylation of active KaiC that is stimulated by KaiA. The reactions in Eq. S3 model the binding of KaiB to inactive KaiC, and those in S4 model the sequestration of KaiA by inactive KaiC that is bound to KaiB; note that in this model an inactive KaiC hexamer can bind up to two KaiA dimers. The reactions in Eqs. S5 and S6 model

spontaneous phosphorylation and dephosphorylation of active and inactive KaiC. For a more detailed discussion of the model, we refer to [25].

The TTC and the coupling between the PPC and TTC are described by the following reactions:

$$\widetilde{\mathrm{R}} + \mathrm{X} \xrightarrow{k_{\mathrm{a}}} \mathrm{R} + \mathrm{X}, \qquad \mathrm{R} + \widetilde{\mathrm{X}} \xrightarrow{k_{\mathrm{i}}} \widetilde{\mathrm{R}} + \widetilde{\mathrm{X}}, \tag{S7}$$

$$\emptyset \underset{\tau}{\overset{\beta \tilde{G}(t)[\mathrm{R}]^4/(K^4+[\mathrm{R}]^4)}{\Longrightarrow}} \mathrm{C}_6 + 3\mathrm{B}, \qquad \emptyset \xrightarrow{\beta_{\mathrm{a}}} \mathrm{A},\, \emptyset \xrightarrow{\beta_{\mathrm{r}}} \widetilde{\mathrm{R}}, \tag{S8}$$

$$\mathrm{R}, \widetilde{\mathrm{R}}, \mathrm{A}, \mathrm{B}, \mathrm{AC}_i, \mathrm{B}_x\widetilde{\mathrm{C}}_i, \mathrm{A}_y\mathrm{B}_x\widetilde{\mathrm{C}}_i \xrightarrow{\mu} \emptyset\,. \tag{S9}$$

Here, R and $\widetilde{\mathrm{R}}$ denote the RpaA protein in its active and its inactive form, respectively. The X and $\widetilde{\mathrm{X}}$ in Eq. (S7) denote any of the phosphoforms of KaiC that mediate the activation and repression of RpaA, respectively; as described in more detail in [35], KaiC in the phosphorylation phase activates RpaA, while KaiC in the dephosphorylation phase deactivates it. The double arrow indicates a reaction with a fixed delay $\tau$; we use $\tau$ rather than $\Delta$ to denote the delay to agree with the notation of [35]. We thus assume that *kaiBC* expression is activated by RpaA and that the activity of RpaA is modulated by the PPC. In contrast, the expression of KaiA and RpaA is taken to occur constitutively. The effect of gene replication is included by making the rate of $\mathrm{C}_6$ production dependent on $\tilde{G}(t)$, just as in the NTFO.

We use the parameters given in the supplementary information of [35], except for: $\beta = 1.02 \cdot 10^2 \mathrm{h}^{-1}$ and $\mu_{\mathrm{tot}} = 0.1\mathrm{h}^{-1}$. As for the NTFO, we keep the total degradation rate constant, so that we can distinguish the effects of protein dilution from those due specifically to periodic gene replication events.

## III. TTC COMBINED WITH A PPC FROM RUST 2007 (FIG. S9)

We argue in the main text that entrainment of circadian clocks by the cell cycle should be a robust, generic phenomenon that does not depend on the precise model studied. In support of this claim, we here study a model of the Kai system proposed by Rust *et al.* [26]. This model describes the PPC at the level of KaiC monomers, rather than of hexamers, as in the model of Zwicker et al. considered in the preceding section and in the main text [35] (which in turn is based on that of Van Zon and coworkers [25] ). The monomers go through a sequence of 4 different phosphorylation states—unphosphorylated (U), phosphorylated only on threonine 432 (T), doubly phosphorylated (D), and phosphorylated only on serine 431 (S)—in a 24 hour cycle [37]. As detailed in the supplementary information of [35], we extended the original Rust model, which contains only the PPC, to include a transcription-translation cycle. Here, we briefly describe the model and discuss how it responds to forcing from the cell cycle.

This PPC is described by the reactions

$$\mathrm{U} \leftrightarrow \mathrm{T}, \qquad \mathrm{T} \leftrightarrow \mathrm{ST}, \qquad \mathrm{ST} \leftrightarrow \mathrm{S}, \qquad \mathrm{S} \leftrightarrow \mathrm{U} \tag{S10}$$

with reaction rates given by Eq. 5 of the supplementary material of Rust *et al.* [26]. These rates depend on the concentration of free KaiA, which is sequestered by KaiC in the S-state. We model KaiA sequestration explicitly:

$$\mathrm{S} + \mathrm{A} \leftrightarrow \mathrm{AS}, \qquad \mathrm{AS} + \mathrm{A} \leftrightarrow \mathrm{A}_2\mathrm{S}. \tag{S11}$$

Dephosphorylation of KaiC in the S-state is allowed to occur even when KaiA is bound, in which case the KaiA protein is released from the complex. We define the output signal as

$$p(t) = \frac{[\mathrm{T}] + [\mathrm{ST}] + [\mathrm{S}] + [\mathrm{AS}] + [\mathrm{A}_2\mathrm{S}]}{[\mathrm{U}] + [\mathrm{T}] + [\mathrm{ST}] + [\mathrm{S}] + [\mathrm{AS}] + [\mathrm{A}_2\mathrm{S}]}, \tag{S12}$$

which resembles the phosphorylation ratio in the case where we cannot distinguish between singly and doubly phosphorylated KaiC. The denominator in the above expression is also the total KaiC monomer concentration. We use the same total protein concentrations as Rust *et al.*, [KaiA] = 1.3 $\mu$M (active KaiA monomers) and [KaiC] = 3.4 $\mu$M (KaiC monomers).

The TTC is modeled as:

$$\emptyset \underset{\tau}{\overset{\beta \tilde{G}(t)[\mathrm{R}]^4/(K^4+[\mathrm{R}]^4)}{\Longrightarrow}} \mathrm{ST}, \quad \emptyset \xrightarrow{\beta_a} \mathrm{A}, \emptyset \xrightarrow{\beta_r} \widetilde{\mathrm{R}}, \tag{S13}$$

$$\widetilde{\mathrm{R}} + \mathrm{T} \xrightarrow{k_a} \mathrm{R} + \mathrm{T}, \quad \mathrm{R} + \mathrm{A}_x\mathrm{S} \xrightarrow{k_i} \widetilde{\mathrm{R}} + \mathrm{A}_x\mathrm{S}, \qquad x \in \{0, 1, 2\}, \tag{S14}$$

$$\mathrm{A}, \mathrm{R}, \widetilde{\mathrm{R}}, \mathrm{U}, \mathrm{S}, \mathrm{A}_x\mathrm{S}, \mathrm{T}, \mathrm{ST} \xrightarrow{\mu} \emptyset. \tag{S15}$$

The first line describes protein production and decay; as in Eq. S9, the double arrow indicates a delayed reaction. The second line summarizes the RpaA signaling pathway, where KaiC that is phosphorylated at the T site activates RpaA and KaiC that is phosphorylated at the S site represses RpaA activation.

As in our other models, we introduced the effect of gene replication by making the production rate of KaiC proportional to the production density $\tilde{G}(t)$. We use the parameters given in [26] and in section S5.2 of the supplementary information of [35], except for $\beta = 1.29 \cdot 10^3 \mathrm{h}^{-1}$ and $\mu_{\mathrm{tot}} = 0.1\mathrm{h}^{-1}$.

Fig. S9 shows the peak-to-peak times of the phosphorylation fraction of this model as a function of the cell-division time $T_{\mathrm{d}}$. Clearly, a model combining a TTC with a PPC based on the Rust model [26] responds to forcing from the cell cycle in essentially the same way as the Zwicker TTC-PPC model [35], supporting the idea that the benefit of a self-contained protein-modification oscillator is a generic feature of biological clocks.

## IV. THE NEGATIVE TRANSCRIPTIONAL FEEDBACK OSCILLATOR WITH INTRINSIC NOISE (FIG. S1)

To test the effect on the locking mechanism of intrinsic noise in the chemical reactions that constitute the circadian clock, we simulate the negative transcriptional feedback oscillator (NTFO) using kinetic Monte Carlo simulations of the chemical master equation. Eq. 2 of the main text implies that when this intrinsic noise is neglected, the number of proteins $N_{\mathrm{C}}$ in the cell obeys

$$\frac{dN_{\mathrm{C}}(t)}{dt} = \beta g(t-\Delta)\frac{K_{\mathrm{C}}^2}{K_{\mathrm{C}}^2 + \left(\frac{N_{\mathrm{C}}(t-\Delta)}{V(t)}\right)^2} - \mu_{\mathrm{act}} N_{\mathrm{C}}(t). \tag{S16}$$

Here, $V(t)$ is the cell volume, which grows exponentially as described in the main text, and $\mu_{\mathrm{act}}$ is the active contribution to the total decay rate $\mu_{\mathrm{tot}} = \mu_{\mathrm{act}} + \mu_{\mathrm{d}}$ in Eq. 2; the term $\mu_{\mathrm{d}}$ contributes to the total apparent decay rate for the protein concentration, but not for the protein number. To include the effects of intrinsic noise on the evolution of $N_{\mathrm{C}}$, we adapted the standard kinetic Monte Carlo algorithm to take into account delayed reactions, volume growth, and gene replication, as described in [35]: The cell volume is increased at discrete time intervals, and reaction propensities are re-calculated after each volume update. After each cell division, the protein number $N_{\mathrm{C}}$ is chosen from a binomial distribution, with $N_{\mathrm{C}}$ halved on average. Gene replication is included through the time dependence of the gene copy number $g(t)$, whose behavior is detailed in the main text.

The parameters used in the simulation are: $\beta = 6.0 \cdot 10^3 \mathrm{h}^{-1}$; $K_c = 1.0\mu\mathrm{M}$; $n = 2$; $\Delta = 8\mathrm{h}$. The time average $\bar{V}$ of the cell volume is chosen to be $1\mu\mathrm{m}^3$. For different cell division times $T_{\mathrm{d}}$, we change the active degradation rate such that the total decay rate is kept constant at $0.2\mathrm{h}^{-1}$: $\mu_{\mathrm{act}} = 0.2\mathrm{h}^{-1} - \log(2)/T_{\mathrm{d}}$. As in the main text, this allows us to disentangle the effect of gene replication on locking from that of simple protein dilution.

We vary the cell division time $T_{\mathrm{d}}$ from 6 to 52 hours in 0.1 hour intervals and simulate a single trajectory of 10,000 hours for each $T_{\mathrm{d}}$. From the trajectories, we extract the peak-to-peak times of the oscillations (see Methods in this document). Fig. S1 shows the average peak-to-peak time of the stochastic NTFO for different values of the cell division time, with initial gene copy number $N = 1$. Two differences from Fig. 2 of the main text, where the system obeys deterministic equations, are worthy of note: First, the 1:1 locking region is much larger when intrinsic noise is included, while the width of the 2:1 locking region has decreased. Intrinsic noise can thus dramatically change the extent of locking. We leave a full investigation of the origins of this effect for future work. Second, because of intrinsic noise, the amplitude is considerably more variable, and the variances in the peak-to-peak times outside of the locking regions are much larger. As in the mean-field model, the variances are very small around $T_{\mathrm{d}} = 24$ hrs, due to locking.

## V. THE EFFECT OF NOISE IN THE TIMING OF GENE REPLICATION EVENTS (FIG. S2)

In the model of the cell cycle described in the main text, gene replication events occur at perfectly regular, evenly spaced intervals in time. In this section, we explore how stochastic variability in the timing of these replications affects the interaction between the cell cycle and other oscillators. We consider a model in which each gene replicates exactly once in each cell division cycle, at a time $t_{\mathrm{g}}$ between 0 and $T_{\mathrm{d}}$, where $T_{\mathrm{d}}$ is the length of the cell cycle and does not vary. The times $t_{\mathrm{g}}$ are drawn in each cell cycle independently from a Gaussian distribution of mean $\bar{t}_{\mathrm{dup}} = T_{\mathrm{d}}/2$ and variance $\sigma_{\mathrm{dup}}^2$. Replication times $t'_{\mathrm{g}}$ that fall outside the interval $[0,T_{\mathrm{d}})$, are mapped back onto it via $t_{\mathrm{g}} = \mathrm{Mod}(t'_{\mathrm{g}}, T_{\mathrm{d}})$.

We assume that the standard deviation in the gene replication times, $\sigma_{\mathrm{dup}}$, is proportional to the cell division time: $\sigma_{\mathrm{dup}} \propto T_{\mathrm{d}}$. Because this quantity is, to our knowledge, not known for *S. elongatus*, we varied this quantity between zero and a value that corresponds to replication times being chosen randomly from a uniform distribution, $\sigma_{\mathrm{dup}}/T_{\mathrm{d}} = 1/\sqrt{12} \approx 0.3$.

Fig. S2 shows the effects of introducing this variability on the behavior of our clock models. For the NTFO (Fig. S2A), the locking regions are reduced in size, but still clearly noticeable. The variance in the peak-to-peak times is typically larger than in deterministic case. For the TTC-PPC model of Zwicker [35] (Fig. S2B), the locking regions have almost disappeared, but the variance in $T_{\rm PtP}$ is nearly unaffected by the noise in the timing of gene replication. Panel C shows representative time traces of the total KaiC concentration, $C_{\rm tot}(t)$ and the phosphorylation fraction $p(t)$, for $T_{\rm d} = 48$h. Clearly, $C_{\rm tot}(t)$ shows much more variability in the height of its peaks than does $p(t)$, further demonstrating the value of a post-translational oscillator in insulating a circadian clock from influences from the cell cycle. We also note that, as in the deterministic limit, the amplitude of the $C_{\rm tot}$ oscillation cycles still (despite the noise) alternates between a high and a low value when gene replications occur only once every 48 hours. It should thus be possible to observe experimentally that $C_{\rm tot}(t)$ is markedly affected by periodic gene replication, while $p(t)$ is much less so.

## VI. ALLOWING THE PROTEIN DECAY RATE TO VARY WITH GROWTH RATE (FIG. S3)

The total protein decay rate $\mu_{\rm tot}$ depends on the rate of active protein degradation $\mu_{\rm act}$ and on the rate of dilution due to cell growth $\mu_{\rm d}$. In the results shown in the main text, we adjusted the active degradation rate with the growth rate so that the total protein decay rate remained constant—this allowed us to zoom in on the effect of locking that is due to periodic gene replication while ignoring confounding changes to clock behavior that might arise because of the variation of $\mu_{\rm tot}$.

It is entirely possible, however, that the real clock system in *S. elongatus* is actually closer to the opposite limit, in which $\mu_{\rm act}$ is fixed and $\mu_{\rm d}$ and $\mu_{\rm tot}$ vary together with the division time $T_{\rm d}$. To investigate how this affects the locking mechanism, we performed simulations in which we kept the active degradation rate $\mu_{\rm act}$ constant, but allowed the total degradation rate $\mu_{\rm tot}$ to vary with the cell-divisition time: $\mu_{\rm tot} = \mu_{\rm act} + \ln(2)/T_{\rm d}$; upon varying $\mu_{\rm tot}$, we adjusted the protein synthesis rate $\beta$ to keep the oscillation period at 24 h. The result is shown in Fig. S3. Just as in the case in which $\mu_{\rm tot}$ is fixed, the effect of locking is very pronounced, both for a simple NTFO (panel A) and for a clock incorporating both a TTC and a PPC (panel B).

## VII. HOW DOES THE CELL READ OUT THE PHOSPHORYLATION FRACTION INSTEAD OF THE CONCENTRATION OF KAIC? (FIG. S4)

Both Fig. 4 and a comparison of the blue lines in Figs. S2A,B show that a circadian clock with a post-translational oscillator is much more robust to a time-varying gene density than is an NTFO. Both the peak-to-peak time and the amplitude of the phosphorylation fraction $p(t)$ of the PPC-TTC vary considerably less not just than the corresponding quantities for the NTFO, but even than those for the total protein concentration $C_{\rm tot}(t)$ of the PPC-TTC itself. To take advantage of the relative stability of the oscillation in $p(t)$, the cell needs to read out the phosphorylation fraction in a way that is insensitive both to the total concentration of KaiC and to the absolute concentrations of its specific phosphorylation states. How does it accomplish this?

To find out, we looked at the architecture of the biochemical network in *S. elongatus* that allows the clock to regulate the transcription of downstream genes. The temporal information encoded in the dynamics of the clock proteins is transmitted via a central node, the response regulator RpaA. This protein can be phosphorylated, and it is known that the phosphorylation level of RpaA controls the expression not only of core clock components, but also of a small set of genes that, in turn, direct genome-wide circadian rhythms [30, 33]. The phosphorylation state of RpaA is regulated by a push-pull network consisting of the histidine kinases SasA, which acts primarily to phosphorylate RpaA, and CikA, whose primary function is to dephosphorylate it [30–32]. The activities of SasA and CikA are in turn controlled by the different phosphorylation states of KaiC, such that KaiC proteins that are in the phosphorylation phase of the clock tend to push up the phosphorylation level of RpaA [30], while those that are in the clock's dephosphorylation phase tend to pull down RpaA's phosphorylation level [31].

To show that such a push-pull network makes the clock readout, the RpaA phosphorylation level, sensitive to the KaiC phosphorylation fraction $p(t)$, but not to its concentration $C_{\rm tot}(t)$, we adapted the canonical model of Goldbeter and Koshland [38]. A cartoon of the model is shown in Fig. S4B. It consists of a substrate S, playing the role of RpaA, which can be phosphorylated and dephosphorylated by the antagonistic enzymes K and P, corresponding respectively to SasA and CikA, each of which can be in active (K$^*$ and P$^*$) or inactive states. Transitions between these states are governed by the time-dependent forward rates $k_{\rm K}(t)$ and $k_{\rm P}(t)$, which mimic the effects of time-varying concentrations of different KaiC phosphoforms. In our model, KaiC in the phosphorylation phase increases $k_{\rm K}(t)$, while KaiC in the dephosphorylation phase increases $k_{\rm P}(t)$. The substrate-modification reactions follow the standard Michaelis-Menten schemes $\rm K^* + S \rightleftharpoons K^*S \rightarrow K^* + S_p$ and $\rm P^* + S_p \rightleftharpoons P^*S_p \rightarrow P^* + S$.

The key question is whether the phosphorylation level of RpaA depends only on the phosphorylation fraction of KaiC, $p(t)$, or whether it is also significantly affected by the total concentration of KaiC. In terms of the model just presented, we must thus ask whether $[S_p]/[S_{tot}]$ (the fraction of phosphorylated RpaA) is sensitive only to the *ratio* $k_K(t)/k_P(t)$ or whether it depends on the two rates individually. We begin by considering this question for the case of time-independent rates, in which case the ratio of total concentrations of the active enzyme forms $[K^*]/[P^*]$ is proportional to $k_K(t)/k_P(t)$ and may be used in its place. In qualitative terms, it is easy to imagine that, since $K^*$ and $P^*$ have opposite effects, increasing the concentration of each one by the same factor might speed up the reaction kinetics but would not affect the steady state ratio $[S_p]/[S_{tot}]$. Indeed, in the regime that the concentrations of the complexes $K^*S$ and $P^*S_p$ are negligible compared to the concentrations of free S and $S_p$, we can equate the rates of S phosphorylation and dephosphorylation in steady state to arrive at a relation of the form

$$\frac{k_+[K^*][S]}{K_{M,+}+[S]} = \frac{k_-[P^*][S_p]}{K_{M,-}+[S_p]} \,. \tag{S17}$$

Together with the conservation law $[S]+[S_p]=[S_{tot}]$, this equation can easily be solved to give $[S_p]/[S_{tot}]$ as a function of $[K^*]/[P^*]$ only. It is possible, however, that in the RpaA system the concentrations of the intermediate complexes $K^*S$ and $P^*S_p$ cannot be neglected. Fig. S4A shows that even in this case, to a very good approximation the steady state phosphorylation fraction of S depends only on the ratio $[K^*]/[P^*]$. This mechanism, by which the output of a push-pull network depends on the ratio of the concentrations of the two antagonistic enzymes, but not on their absolute values, has previously been invoked to explain the robustness of the *E. coli* chemotaxis pathway to concerted variations in the expression levels of the chemotaxis proteins [43].

To extend these results to the case of time-varying activation rates that is more directly relevant to a situation in which the concentrations of the KaiC phosphoforms rise and fall, we allow $k_K(t)$ and $k_P(t)$ to vary with time as shown in Fig. S4C (upper graph): Similarly to the total KaiC concentration at $T_d = 48$ hours with $N = 1$ (Fig. 4C of the main text), each rate changes periodically with a period of 48 hours, with alternating higher and lower peaks. The lower graph of Fig. S4C , with time traces of $[S_p]$, $[K^*]$ and $[P^*]$, shows that even though the amplitude of $[K^*](t)$ and $[P^*](t)$ varies between oscillation cycles, the amplitude of $S_p(t)$ is constant. Comparable behavior is expected as long as the rates associated with the enzymatic reactions are faster than the timescale of variation of $k_K(t)$ and $k_P(t)$. Provided this is the case, the push-pull system built around RpaA will allow the bacterium to take as its clock readout the phosphorylation fraction $p(t)$—which we have argued is robust to perturbations associated with the cell cycle—rather than the absolute concentration of KaiC or one of its phosphoforms.

## VIII. MULTIPLE CHROMOSOMES REDUCE THE COUPLING STRENGTH IN BOTH THE PPC-TTC AND THE NTFO (FIG. S5)

Fig. 5C of the main text shows the average peak-to-peak time and its standard deviation for the PPC-TTC model of Zwicker *et al.* [35] as a function of the cell-division time $T_d$, both for $N = 1$ and for $N = 4$. Panel A of Fig. S5 shows exactly the same figure, but with underneath it, for $N = 4$, time traces for $p(t)$ and $C_{tot}(t)$ at $T_d = 24.5$ h (panel B) and $T_d = 48$ h (panel C), as also indicated by the arrows in panel A. As discussed in the main text, the effects of the cell cycle have almost completely disappeared, even at $T_d = 24.5$ h, immediately outside the locking regime, where the effects are usually most visible.

Panels D–G of Fig. S5 show the effect of multiple chromosomes on the locking behavior of the NTFO. Panel D shows that with $N = 4$ chromosome copies at the beginning of the cell cycle, both the variance and the width of the locking regions have decreased to no more than one hour. The time traces (Fig. S5E–G) of the protein concentration at cell division times of 24, 27 and 48 hours confirm that the NTFO has indeed become very stable. At $T_d = 27$ hours, where the protein concentration had showed irregular behavior and large amplitude variations for $N = 1$, its behavior has now become much more regular. At a division time of 48 hours, the marked amplitude variations present when $N = 1$ have disappeared. Indeed, the beneficial effect of a higher gene-copy number is larger than that of adding a PPC, as can be seen by comparing Fig. S5D with Fig. 4 of the main text. Of course, the most stable clock is obtained when a higher gene copy number is combined with a PPC (see Fig. 5), suggesting that both are needed for circadian rhythms that are maximally resilient against perturbations from the cell cycle.

## IX. PHASE DIAGRAMS FOR THE NTFO AND THE MODELS BY ZWICKER ET. AL. AND RUST ET. AL. (FIG. S6)

In order to get a better understanding of how the cell cycle perturbs the clock, we have made phase diagrams for both the width of the 1:1 locking region and the average variance of the peak-to-peak times, as a function of the two

key variables that affect locking, the number of gene copies $N$ and the standard deviation in their replication times, $\sigma_{\rm dup}$, for all models, *i.e.* the NTFO model, the TTC-PPC model of Zwicker *et al.* [35] and the model that combines a TTC with the PPC of Rust *et al.* [26, 35], hereafter referred to as the Rust model.

To make phase diagrams as a function $N$ and $\sigma_{\rm dup}$, we need to extend our model of stochasticity in the timing of gene replication introduced earlier in this document for $N = 1$, to also allow for a higher gene copy number, $N > 1$. Each cell cycle has $N$ gene replication events which occur at times $t^i_{\rm g}$ within the interval [0,$T_{\rm d}$). Each replication time is drawn from a Gaussian distribution with a standard deviation $\sigma_{\rm dup}$ that is proportional to $T_{\rm d}$, and a mean $\bar{t}^i_{\rm g} = T_{\rm d}/N(\frac{1}{2} + i)$, where $i \in \{0, \ldots, N-1\}$ for each cell cycle. Replication times $t'^i_{\rm g}$ that fall outside the interval [0,$T_{\rm d}$), are mapped back onto it via $t^i_{\rm g} = {\rm Mod}(t'^i_{\rm g}, T_{\rm d})$. Note that this mapping slightly decreases the variance in the replication times; the real variance will therefore be slightly less than $\sigma^2_{\rm dup}$ (at most 10%).

We run simulations with values for $\sigma_{\rm dup}/T_{\rm d}$ in the range $[0, 0.3]$, which, as mentioned above, corresponds to a scenario where the replication time is essentially chosen at random between 0 and $T_{\rm d}$. We consider initial gene copy numbers of $N \in \{1, 2, 3, 4\}$.

Panels A, E, and I of Fig. S6 show the phase diagrams of the width of the 1:1 locking regions as a function of $N$ and $\sigma_{\rm dup}/T_{\rm d}$, for the NTFO, Zwicker and Rust models, respectively. The panels underneath, (B, F, J), respectively, show cuts through these phase diagrams. Here, we consider an oscillator to be 1:1 locked to the cell cycle when the difference between its average PtP-time, $\langle T_{\rm PtP}\rangle$, and the cell-division time $T_{\rm d}$ is less than 0.05 hour: $\langle T_{\rm PtP}(T_{\rm d})\rangle - T_{\rm d} < 0.05$.

Panels C, G, K of Figs. S6 show the phase diagrams of the average variance in the peak-to-peak times, $\langle\sigma^2_{\rm PtP}\rangle$, again as a function of $N$ and $\sigma_{\rm dup}/T_{\rm d}$, for the NTFO, Rust and Zwicker models, respectively. Here, the variance is averaged over a range of cell-division times $6 < T_{\rm d} < 52$:

$$\langle\sigma^2_{\rm PtP}\rangle = \frac{1}{N_{\rm sim}} \sum_{i=1}^{N_{\rm sim}} \sigma^2_{\rm PtP}(T^i_{\rm d}), \tag{S18}$$

where $N_{\rm sim}$ is the number of evenly-spaced simulations performed in the range $6 < T_{\rm d} < 52$ in steps of 0.1 hour, and $\sigma^2_{\rm PtP}(T^i_{\rm d})$ is the variance in the PtP-times for 5000 hours of simulated time at cell-divistion time $T^i_{\rm d}$. This quantity is a measure for the erratic behavior induced by the coupling to the cell cycle outside the locking region.

It seen that for all models both the width of the 1:1 locking region (Fig. S6A/B, E/F, I/J) and the variance in the peak-to-peak times (Fig. S6C/D,G/H, K/L), initially rapidly decreases with $N$, but then reaches a plateau. Even in the limit that $N \to \infty$, there is still some weak, residual driving by the cell cycle, because $N$ rises linearly while the volume $V$ rises exponentially during the cell cycle, leading to periodic variations in the gene density $G(t) = N(t)/V(t)$. It is also seen that the width of the 1:1 locking region decreases with increasing $\sigma_{\rm dup}$, especially when $N$ is small. However, while increasing the noise in the timing of replication reduces the width of the locking region, it also strongly increases the variance in the peak-to-peak times. A reliable clock requires not only a small locking window, but also a small peak-to-peak variance. Clearly, allowing for stochasticity in the timing of replication is not a solution to the locking problem.

Comparing the different models, it is seen that building the clock around a PPC reduces not only the width of the locking region, but also the variance in the peak-to-peak times, both in the Zwicker (Fig. S6E–H) and in the Rust model (Fig. S6I–L). However, with $N = 1$ chromosome copy at the beginning of the cell cycle, the introduction of the PPC is not sufficient to fully eliminate locking. A TTC-PPC model still requires multiple chromosome copies that are replicated asynchronously.

## X. TWO SYNTHETIC OSCILLATORS: THE REPRESSILATOR AND THE DUAL-FEEDBACK OSCILLATOR (FIGS. S7–S8)

While in the main text we focus on circadian clocks, the mechanism of entrainment via periodic gene replication is very generic, and should thus pertain to any cellular oscillator, including synthetic oscillators. To investigate this, we study how strongly two canonical synthetic oscillators, both constructed in *E. coli*, can lock to the cell cycle: the repressilator, developed by Elowitz and Leibler [49], and the dual-feedback oscillator, developed by Hasty and coworkers [50]. Importantly, these synthetic oscillators were originally constructed on plasmids, which often occur in large copy numbers: the plasmid copy number of the dual-feedback oscillator, for example, has been estimated to be around 25 [50]. Moreover, experiments indicate that these plasmids are copied at random times during the major part of the cell cycle [54]. In line with our observation that multiple chromosome copies that are replicated asynchronously strongly reduce the strength of locking (Fig. 5 of the main text and Fig. S6), we find that with multiple (i.e. $N = 25$) asynchronously replicating plasmids, these synthetic oscillators lock to the cell cycle only very weakly: both the width of the 1:1 locking region and the variance in the peak-to-peak time are less than a percent of their respective average. Interestingly, the deterministic simulations show that even in the limit $N \to \infty$, very

weak locking can still be observed. This can be understood by noting that in this limit $N$ rises linearly over the cell cycle, while $V$ grows exponentially, which means that the gene density $G(t) = N(t)/V(t)$ exhibits (small) periodic variations. However, in this limit locking is indeed very weak, and most likely impossible to detect experimentally. We thus expect that with multiple asynchronously replicating plasmids, locking of these synthetic oscillators to the cell cycle is difficult, if not impossible, to detect experimentally.

However, synthetic networks are increasingly being constructed directly onto the chromosome. If the repressilator and dual-feedback oscillator were similarly integrated into the chromosome of *E. coli*, then strong coupling to the cell cycle can be expected, as we will show below. *E. coli* typically has one chromosome at the beginning of the cell cycle, in which case the gene copy number goes from 1 to 2 over the course of the cell cycle. At high growth rates, corresponding to cell division times shorter than the replication time of the DNA (on the order of 40 minutes), the chromosome can have multiple replication forks, which means that the gene copy number can be larger. Here, however, we only consider the regime that the cell division time is on the order of the DNA replication time or longer, such that the gene copy number rises from $N = 1$ at the beginning of the cell cycle to $2N = 2$ at the end. Interestingly, both synthetic oscillators consist of more than one gene, in contrast to the NTFO of the main text. Moreover, the period of both synthetic oscillators can be on the order of the cell cycle time and the DNA replication time. This means that the spatial distribution of the genes on the chromosome can become critically important, as we will show below.

**Repressilator (Fig. S7)** The repressilator consists of three genes, where the first gene represses the expression of the second, which represses the third gene, which in turn represses the expression of the first again [49]. To take into account gene replication, we change the model of Elowitz and Leibler by making the expression of the mRNA proportional to the gene density $G_i(t)$:

$$\frac{dm_i(t)}{dt} = -m_i(t) + \frac{G_i(t)}{\bar{G}_i}\frac{\alpha}{1+(p(t)_j)^n} + \alpha_0 \tag{S19}$$
$$\frac{dp_i(t)}{dt} = -\mu_p p_i(t) + \gamma m_i(t)$$

Here, $m_i$ and $p_i$ are the concentrations of mRNA and proteins ($i \in \{1, 2, 3\}$), both rescaled with the constant of half-maximum repression $K_M$. Since transcription is fast compared to the clock period, the delay $\Delta$ in the expression of the mRNA is ignored—the transcription rate is thus assumed to be proportional to the instantaneous gene density $G_i(t)$; importantly, the gene density can differ between the three genes when they are positioned differently on the chromosome. $\bar{G}_i$ is the time-averaged gene density, which depends on the phase of the cell cycle at which the gene is duplicated. The mRNA expression has a basal rate $\alpha_0$ and an enhanced rate $\alpha$, which is repressed by protein $p_j$, where $j \in \{3, 1, 2\}$, with a Hill coefficient $n$; here, following the original paper [49], time is rescaled in units of the mRNA lifetime and protein concentrations are in units of the concentration necessary for half-maximal repression. In the second equation, $\mu_p$ is the protein decay rate over the mRNA decay rate and $\gamma$ is the translation efficiency, *i.e.* the average number of proteins produced per mRNA molecule. We used the parameters given in Box 1 of Ref. [49].

We first consider the scenario in which the three genes are close together on the chromosome, such that we can assume that their genes are replicated at the same time. Fig. S7 shows that in this case the locking is not very strong—the locking windows are very small; the only effect of locking is that in these very small windows the variance in the peak-to-peak time is strongly reduced. The reason why locking is weak is that while the genes are replicated at the same time, they are expressed at different times. This means that gene replication has a different effect on the expression level of each of the three genes. Hence, even when the cell cycle period is approximately equal to the the oscillator's intrinsic period, $T_\text{d} \approx T_\text{int}$, the oscillation of each protein concentration has a different amplitude, as shown in Fig. S7B. This makes it harder for all three protein oscillations to get the same period as that of the cell cycle, and become locked to it. Interestingly, Fig. S7C shows that when the cell-cycle time is twice the intrinsic clock period, the pattern of alternating smaller and larger oscillation amplitudes can still be observed for each of the respective protein concentration profiles. As for the circadian clocks studied in the main text, we believe that this observation can be used to detect the effect of periodic gene replication experimentally.

We now consider a scenario in which the different genes are replicated at different times during the cell cycle, which corresponds to a situation where the genes are located at different positions on the chromosome. We assume that the gene for protein $p_1$ is replicated halfway through the cell cycle, at a time $d_1 = 0$; the gene for $p_2$ is replicated with a delay $d_2$ with respect to the replication of $p_1$; the gene for $p_3$ is replicated at a time $d_3 = -d_2$. Thus the gene for $p_3$ is replicated before that for $p_1$ when $d_2 > 0$, and after that for $p_1$ when $d_2 < 0$. Interestingly, while the locking regions are very small when the genes are replicated at the same time ($d_2 = 0$, panel A, grey lines in panels D and E), replicating them at different times introduces marked locking: both for $d_2 > 0$ (panel D) and $d_2 < 0$ (panel E) strong locking is observed. Even more strikingly, the 1:1 locking region is largest when $d_2 < 0$, meaning $p_2$ is replicated before $p_1$, which is replicated before $p_3$ (panel E). This can be understood by noting that in this case the genes are

replicated in the same temporal order as that in which they are expressed in the oscillator (see panel B): shifting the phase of the clock with respect to that of the cell cycle has then the strongest effect on the amplitude and hence the period of the clock oscillations, which underlies the phenomenon of locking (see Fig. 3 of the main text).

In summary, the repressilator can strongly lock to the cell cycle. Moreover, the strength of locking depends sensitively on when the respective genes are replicated, and hence on their spatial position on the chromosome.

**Dual-feedback oscillator (Fig. S8)** The dual-feedback oscillator consists of two genes, one encoding for an activator and one for a repressor [50]. The activator enhances the expression of both genes, while the repressor represses the expression of both genes. Since the genes have identical promoters, the temporal expression of the two proteins is similar. The model we employ is presented in the SI of [50], but to take into account the periodic variations in the gene density, we have modified the equations describing the transcription of mRNA of the activator and repressor:

$$P_{0,0}^{a/r} \xrightarrow{b_{a/r}G_{a/r}(t)/\bar{G}_{a/r}} P_{0,0}^{a/r} + m_{a/r} \tag{S20}$$
$$P_{1,0}^{a/r} \xrightarrow{\alpha b_{a/r}G_{a/r}(t)/\bar{G}_{a/r}} P_{1,0}^{a/r} + m_{a/r}.$$

Here $P_{m,n}^{a/r}$ denotes the promoter of the (a)ctivator/(r)epressor gene, with $m = 0, 1$ activator protein and $n = 0$ repressor protein bound to it, respectively. The mRNA $m_{a/r}$ of the activator ($a$) and repressor ($r$) is transcribed with a rate $(\alpha)b_{a/r}G(t)$, which depends on the state of the promoter and on the gene density $G_{a/r}(t)$. Because the transcription of mRNA is fast compared to the period of the clock, we neglect the delay $\Delta$ between the beginning and end of transcription. Parameters are given in the SI of Ref.[50], with an arabinose inducer level of 0.7% and a IPTG concentration of 2nM. The intrinsic period of this oscillator without the driving by the gene density is $\sim 40$ minutes. To study the importance of the timing of gene replication, we want an intrinsic period that is longer than the replication time of the DNA, which is also around 40 minutes. To obtain a longer clock period, we use the experimental observation in [50] that the clock period scales with temperature via the Arrhenius law. To this end, we scale all rate constants, $k_i$, in the model, using

$$k_i = k_{\text{ref}} \exp(-\Theta_{\text{cc}}[1/T - 1/T_{\text{ref}}]), \tag{S21}$$

where $k_{\text{ref}}$ is the rate constant at the reference temperature $T_{\text{ref}}$ of 310K and $\Theta_{\text{cc}} \approx 8300$K is a constant. (See SI of [50]). We will evaluate the model at a temperature of 303K where the clock has an intrinsic period of 73 minutes.

Fig. S8A shows the locking of the dual-feedback oscillator with $N = 1$ copy of each gene at the beginning of the cell cycle. We assume here that the genes are located next to each other on the chromosome, so that their time-varying gene-densities are the same. It is seen that the width of the locking regions is much larger than those of the NTFO. In Fig. S8B we show a time trace of the irregular oscillations around a cell-division time of $T_{\text{d}} = 96$ minutes. Fig. S8C shows that, as observed for the circadian clocks studied in the main text, the amplitude of the oscillations alternates between a high and a low value when the cell-division time $T_{\text{d}} = 146$ minutes is about twice the intrinsic clock period, due to periodic gene replication every other clock period. We thus conclude that also the dual-feedback oscillator can strongly lock to the cell cycle when it is constructed onto the chromosome, and that this effect should be observable experimentally.

Fig. S8D,E shows the result of varying the moment of gene replication for the two genes. We let the activator gene always replicate halfway through the cell cycle, and vary the time delay $d_r$ between the replication of the two genes, as $d_{\text{r}} = 0, T_{\text{int}}/12, T_{\text{int}}/8$ and $T_{\text{int}}/4$ (panel D) and minus these values (panel E), where $T_{\text{int}}$ is the intrinsic clock period; panel D corresponds to the case in which the repressor is replicated after the activator, and panel E corresponds to the opposite scenario. It is seen that in both scenarios the strength of locking decreases: the strongest entrainment is observed when the genes are replicated at the same time during the cell cycle (grey lines), in stark contrast to the behavior of the repressilator. Combining the observations on the behavior of the repressilator and the dual-feedback oscillator, the conclusion is that also synthetic circuits can strongly lock to the cell cycle, and that the strength of locking depends very sensitively on both the architecture of the oscillator and on the timing of gene replication and hence on the spatial distribution of the genes on the chromosome.

## XI. METHODS

The delay-differential equations (DDE) describing our models in the absence of noise were propagated using the numerical differential equation solver of Mathematica 8 (Wolfram Research). For each value of $T_{\text{d}}$, we generated a single time trace of 2000 hours. In order to allow the oscillations to settle down to a steady state, we discarded the first 500 hours of each simulation and analyzed the remaining 1500 hours.

To find the peak-to-peak times $T_{\rm PtP}$ in the deterministic DDE simulations (including those with noise in the gene replication times), we used the built-in methods of Mathematica to return all local extrema in the concentration and phosphorylation fraction, respectively; these extrema correspond to the time points $t_i$ where $C_i$ or, respectively, $p_i$, is higher, in the case of a maximum, or lower, in the case of a minimum, than its two immediate neighbors. As is standard for numerical solution of differential equations, the spacing $t_i - t_{i-1}$ between successive time points was determined adaptively by the algorithm to meet imposed precision bounds but never exceeded 0.2 h. We then checked if a given local minimum was the lowest point within an interval of $\pm$ 18 hours centered on the minimum; if so, we defined this point as the global minimum of a single oscillation cycle. If there did exist a local extremum with a lower value, we repeated this procedure around the lower point until we found a point which was the lowest within a time interval of $\pm$ 18 hours. The same procedure was followed for the local maxima. The peak-to-peak time was then calculated by subtracting the times of two consecutive minima; we verified that substracting the times of two consecutive *maxima* gave essentially the same results.

To find the peak to peak times in the kinetic Monte Carlo simulation of the NTFO, we record the protein concentration $c_i(t_i)$ every 0.01 h of simulated time. We then use a sliding window of 18 hours over these concentrations to find the extrema of the oscillations. Specifically, to find the time $t_j$ of the next local minimum: starting from the maximum of the preceding oscillation cycle at time $t_i$, we find the smallest concentration $c_j$, with $j > i$, in the window $t_j - t_i \leq 18$ h. (Given $c_i$ was a local maxmium, there must exist a concentration $c_j < c_i$.) We then check whether there exists a concentration $c_k < c_j$ for $k > j$ and $t_k - t_j \leq 18$ h. If there is, we replace $c_j$ by $c_k$ and again search for a deeper minimum within 18 hours; otherwise, $c_j$ is the minimum of the next oscillation cycle. A completely analogous procedure is used to identify the maxima of successive oscillation cycles.

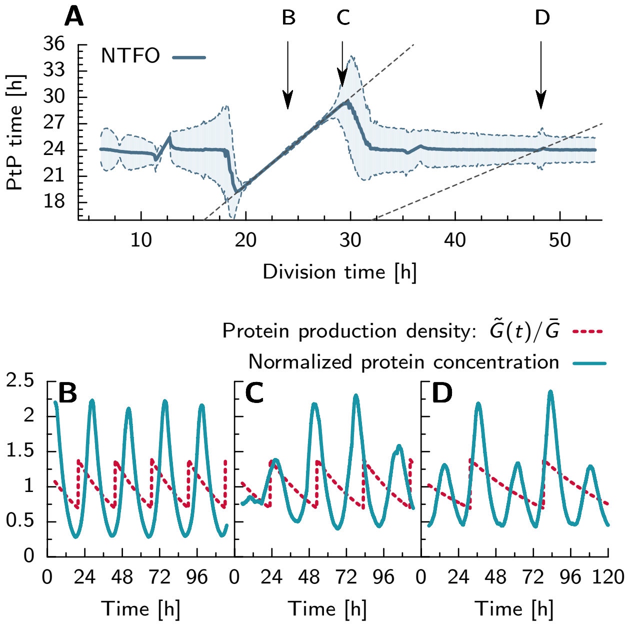


FIG. S1. The effect of intrinsic noise on the locking of the negative transcriptional feedback oscillator (NTFO) to the cell cycle. (A) Average (solid line) and standard deviation (shaded region) of the peak-to-peak time $T_{\mathrm{PtP}}$ as a function of the division time $T_{\mathrm{d}}$ for an NTFO with intrinsic noise and initial gene copy number $N = 1$. The region of 1:1 locking with the cell cycle (left dashed line) has widened considerably compared to the deterministic case (Fig. 2A of the main text), and the standard deviation in $T_{\mathrm{PtP}}$ outside the locking region has increased. In contrast, the region of 2:1 locking (right red dashed line) has shrunk almost to nothing. (B–D) Representative time traces for the division times indicated by the arrows in panel A. Shown are the protein concentration $C(t) = N_C(t)/V(t)$ of the NTFO (blue solid line) and the protein production density $\tilde{G}(t)$ (red dashed line), both normalized by their time average values. At a division time of $T_{\mathrm{d}} = 24$h (B), the NTFO is locked to the cell cycle. Because of the intrinsic noise, the amplitude varies slightly from one oscillation cycle to the next. At $T_{\mathrm{d}} = 27$ h (C), just outside the locking region, the oscillator exhibits irregular behavior. At $T_{\mathrm{d}} = 48$ h (D), the NTFO oscillations switch between a small and a large amplitude in successive oscillation cycles, just as in the deterministic case.

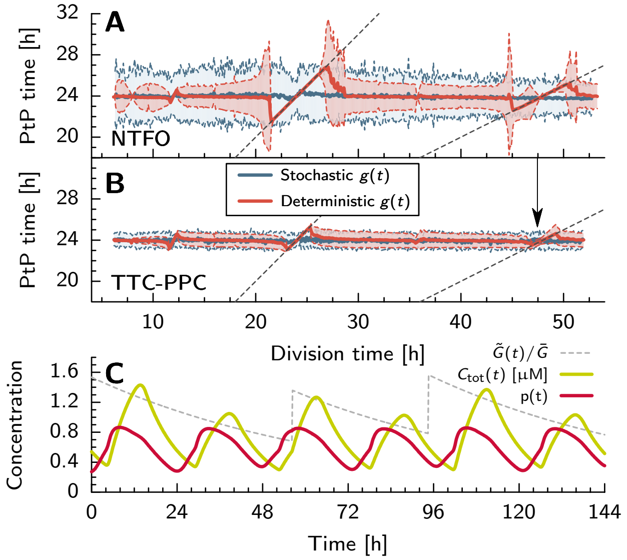


FIG. S2. The effect of stochasticity in the timing of gene replication on locking to the cell cycle. (A) The average and variance of $T_{\rm PtP}$ for an NTFO in which the timing of gene replication is deterministic (red) or is drawn from a Gaussian distribution with a width $\sigma$ that is 30% of the cell-division time $T_{\rm d}$(blue). The stochasticity in the replication times decreases the width of the locking regions, but increases the variance in the peak-to-peak times. (B) Same as A, but for $T_{\rm PtP}$ of the phosphorylation fraction $p(t)$ of the TTC-PPC model of Zwicker *et al.* [35]. Again, stochasticity in the timing of replication reduces locking, but in this case, the increase in the variance of $T_{\rm PtP}$ outside the locking region is much less marked. We attribute this to the ability of the PPC to insulate the clock from variability in gene expression levels. (C) Representative time traces of the production density $\tilde{G}(t)$ (normalized to its time average), the phosphorylation fraction $p(t)$, and the total KaiC concentration $C_{\rm tot}(t)$ for the Zwicker model for $T_{\rm d}$=48h. As in the deterministic limit, the amplitude of the $C_{\rm tot}(t)$ oscillations tends to alternate between a high and a low value, due to gene replication occuring every 48 hours, on average; in contrast, the amplitude of $p(t)$ is relatively constant. The effect of periodic gene replication on $C_{\rm tot}(t)$ should thus be observable experimentally.

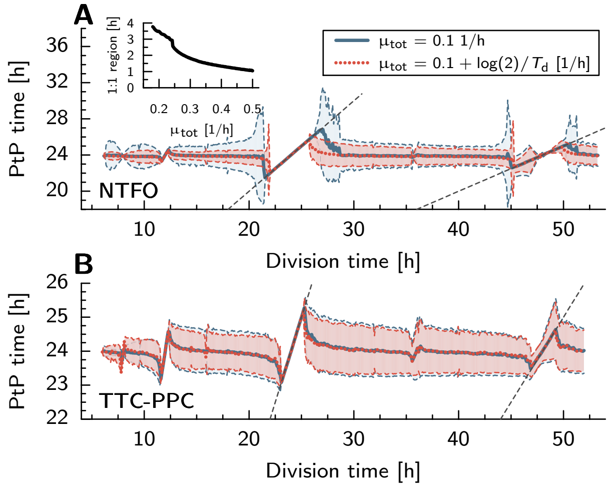


FIG. S3. The effect of allowing the total protein decay rate $\mu_{\rm tot}$ to vary with the cell-division time $T_{\rm d}$, both for an NTFO (A) and for the Zwicker [35] model of a clock that combines a TTC with a PPC (B; note the vertical scale is different than in panel A). The blue lines correspond to the scenario in which the the total degradation rate is kept constant at $\mu_{\rm tot} = 0.1/{\rm h}$ (as in Figs. 2A and 4A of the main text), and the red lines to the scenario in which the total degradation rate depends on the division time as $\mu_{\rm tot} = 0.1{\rm h}^{-1} + \log(2)/T_{\rm d}$ [1/h]. When $\mu_{\rm tot}$ depends on $T_{\rm d}$, we adjust the KaiC production rate $\beta$ such that the intrinsic period of the clock remains 24 hours. For both clock models and both choices of $\mu_{\rm tot}$, the clock tends to lock to the cell cycle. The difference between the results of the two protein-decay scenarios in the case of the NTFO can be understood by noticing that we have chosen our rates so that $\mu_{\rm tot}$ never drops below 0.1 ${\rm h}^{-1}$ in either case, but can become larger than this bound when it is allowed to depend on $T_{\rm d}$. The protein synthesis rate $\beta$ then becomes higher than when $\mu_{\rm tot}$ is constant. The higher synthesis and decay rate raises the amplitude of the concentration oscillations, making the clock more stable. As the inset indicates, the width of the locking region decreases with increasing $\mu_{\rm tot}$ in a similar fashion when $\mu_{\rm tot}$ does not depend on $T_{\rm d}$. The TTC-PPC is almost insensitive to the higher degradation and production rates.

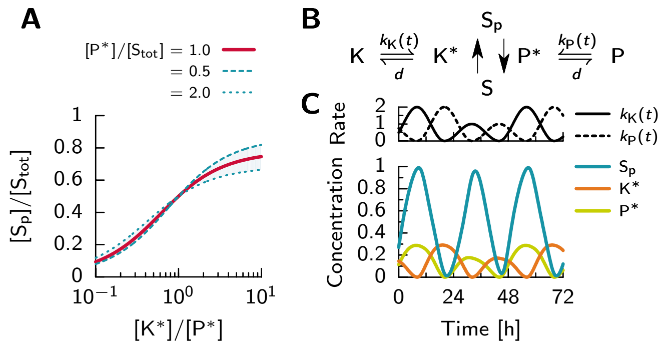


FIG. S4. A push-pull network can read out the phosphorylation fraction $p(t)$ while remaining insensitive to the total concentration $C_{\rm tot}(t)$ of KaiC. (A) Steady-state output of the push-pull network, the fraction of phosphorylated substrate $[\mathrm{S_p}]/[\mathrm{S_{tot}}]$, plotted against the ratio of the active kinase concentration, $[\mathrm{K}^*]$, to the active phosphatase concentration $[\mathrm{P}^*]$; here, $[\mathrm{S_p}]/[\mathrm{S_{tot}}]$ mimics the phosphorylation fraction of RpaA. In steady state (but not necessarily in the general, time-varying case, see panel B) $[\mathrm{K}^*]$ directly reports the concentration of KaiC in the phosphorylation phase of the clock and $[\mathrm{P}^*]$ the concentration of KaiC in the clock's dephosphorylation phase. For the solid red line, we change $[\mathrm{K}^*]/[\mathrm{P}^*]$ from 0.1 to 10, while keeping $[\mathrm{P}^*]$ equal to $[\mathrm{S_{tot}}]$. The dashed and dotted lines show the result when both the kinase and phosphatase concentrations are halved or doubled, respectively. Because of the push-pull architecture, a change in the total concentration $[\mathrm{K}^*] + [\mathrm{P}^*]$ at fixed $[\mathrm{K}^*]/[\mathrm{P}^*]$ has only a small effect on the steady-state level of phosphorylated substrate $[\mathrm{S_p}]/[\mathrm{S_{tot}}]$; the network predominantly responds to the ratio $[\mathrm{K}^*]/[\mathrm{P}^*]$. (B) Schematic of our model of a simple push-pull network. The amount of active kinase, $[\mathrm{K}^*]$, is controlled by the time-dependent rate $k_{\rm K}(t)$ of conversion from K to $\mathrm{K}^*$, and similarly for $[\mathrm{P}^*]$ and $k_{\rm P}(t)$; we imagine that these rates are proportional to the amount of KaiC in the phosphorylation and dephosphorylation phases of the clock, respectively. The two enzymes return to their inactive states at constant rates $d$. The interconversion between S and $\mathrm{S_p}$ follows the standard Michaelis-Menten reaction scheme. (C) Reading out time-varying rates $k_{\rm K}$ and $k_{\rm P}$. (Top) We let $k_{\rm K}(t)$ oscillate with a peak-to-peak time of 24 hours, with the amplitude of each consecutive oscillation cycle changing by a factor of two to mimic the variability in the total amount of KaiC when $T_{\rm d} = 48$ h (Fig. 2 of the main text). $k_{\rm P}(t)$ has the same behavior as $k_{\rm K}(t)$, but phase shifted by 12 hours. (Bottom) With these time-varying inputs, the active enzyme concentrations $[\mathrm{K}^*]$ and $[\mathrm{P}^*]$ track the conversion rates $k_{\rm K}(t)$ and $k_{\rm P}(t)$, but $[\mathrm{S_p}]$ shows an essentially constant amplitude from one cycle to the next. Thus, even with time-varying inputs, the activity of RpaA is sensitive primarily to the ratio $k_{\rm K}(t)/k_{\rm P}(t)$, which plays the role of the phosphoryation ratio $p(t)$, not to each rate individually, or by extention to the absolute concentrations of KaiC phosphoforms. In all calculations, $K_M = [\mathrm{S_{tot}}]$

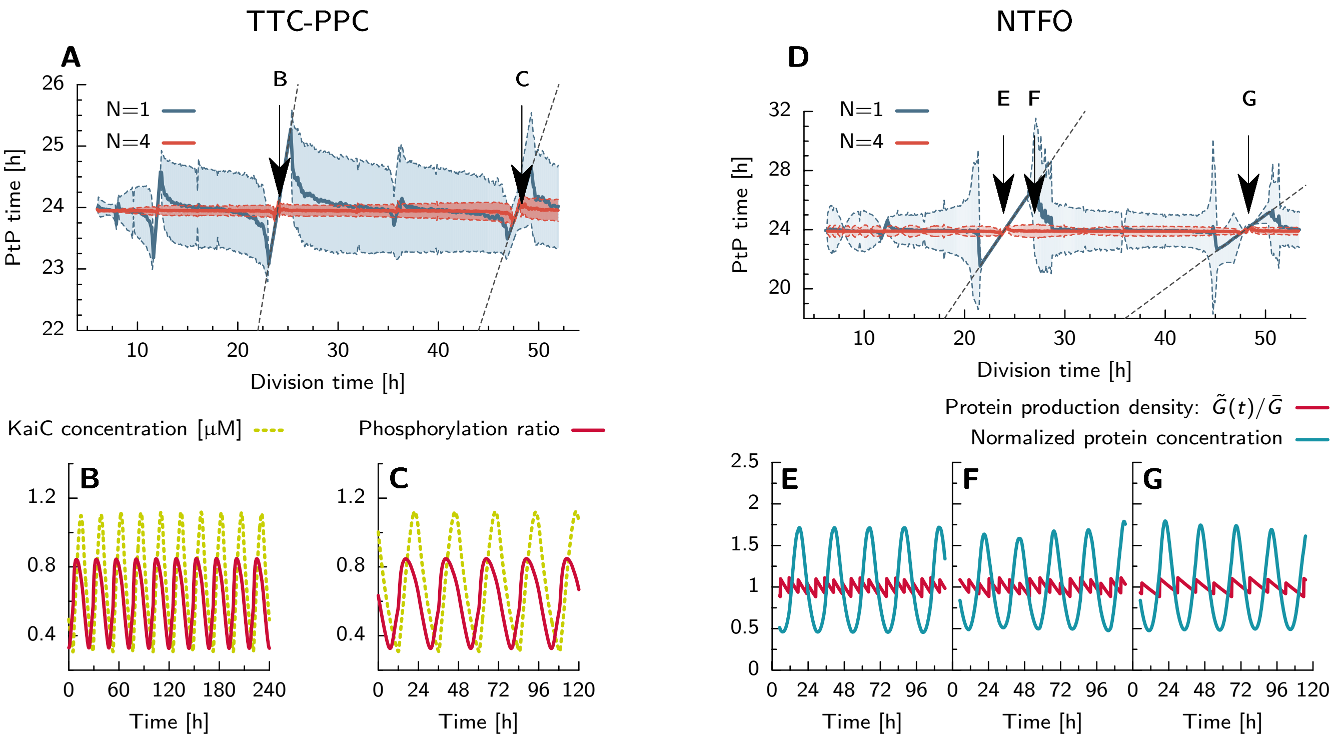


FIG. S5. Multiple chromosome copies reduce the effect of periodic gene replications on both the TTC-PPC oscillator of Zwicker *et al.* [35] (panels A–C) and on the simple negative transcriptional feedback oscillator (NTFO) (panels D–G). Panel (A) shows for the TTC-PPC model the average peak-to-peak time as a function of the cell-division time $T_\mathrm{d}$ for initial gene copy numbers $N = 1$ (blue) and $N = 4$ (red). This panel is identical to Fig. 5C of the main text, except for the arrows indicating the values of $T_\mathrm{d}$ for which times traces are shown in (B,C) for $N = 4$. Both the standard deviation in the peak-to-peak times (given by the shaded regions) and the regions where the oscillator is locked to the cell cycle are strongly reduced for $N = 4$. (B) The total KaiC concentration $C_\mathrm{tot}(t)$ (dashed line) and phosphorylation fraction $p(t)$ (solid line) for the TTC-PPC model at $T_\mathrm{d} = 24.5$ h, for $N = 4$. (C) $C_\mathrm{tot}(t)$ and $p(t)$ at $T_\mathrm{d} = 48$ h for the same model, again for $N = 4$. Note that, even at $T_\mathrm{d} = 24.5$ h, immediately outside the locking region where the variance in $T_\mathrm{PtP}$ is generally largest, the effects of the cell cycle have almost completely disappeared. (D) The average peak-to-peak time and its standard deviation for the NTFO model, for $N = 1$ (blue line) and $N = 4$ (red line). It is seen that as in the Zwicker model, multiple chromosome copies dramatically reduce the strength of locking. (E–G) NTFO time traces of the protein-concentration oscillations $C(t)$ (blue lines) and the production density $\tilde{G}(t)$ (red lines), both normalized to their time average values, for $N = 4$, and for cell-division times indicated by the arrows in (D). With $N = 4$, only at, or very close to $T_\mathrm{d} = 24$ hr (E), is the NTFO locked to the cell cycle. Even at $T_\mathrm{d} = 27$ h (F) and $T_\mathrm{d} = 48$ h (G), where for $N = 1$ the NTFO shows irregular behavior and large amplitude variations, respectively (see Fig. 2C,D), the time courses are much less perturbed by the cell cycle when $N = 4$. However, albeit greatly reduced, the effect of driving by the cell cycle can nonetheless still be observed, both in the persistence of small regions of locking and in the still appreciable variance in $T_\mathrm{PtP}$ when the oscillators are not locked (panel D). A PPC must be added to more fully attenuate the cell cycle's influence. (Compare panel D with panel A, taking into account the difference in scale of the $y$-axis; the standard deviation of $T_\mathrm{PtP}$ is about 3 times larger for the NTFO than for the full TTC-PPC model.)

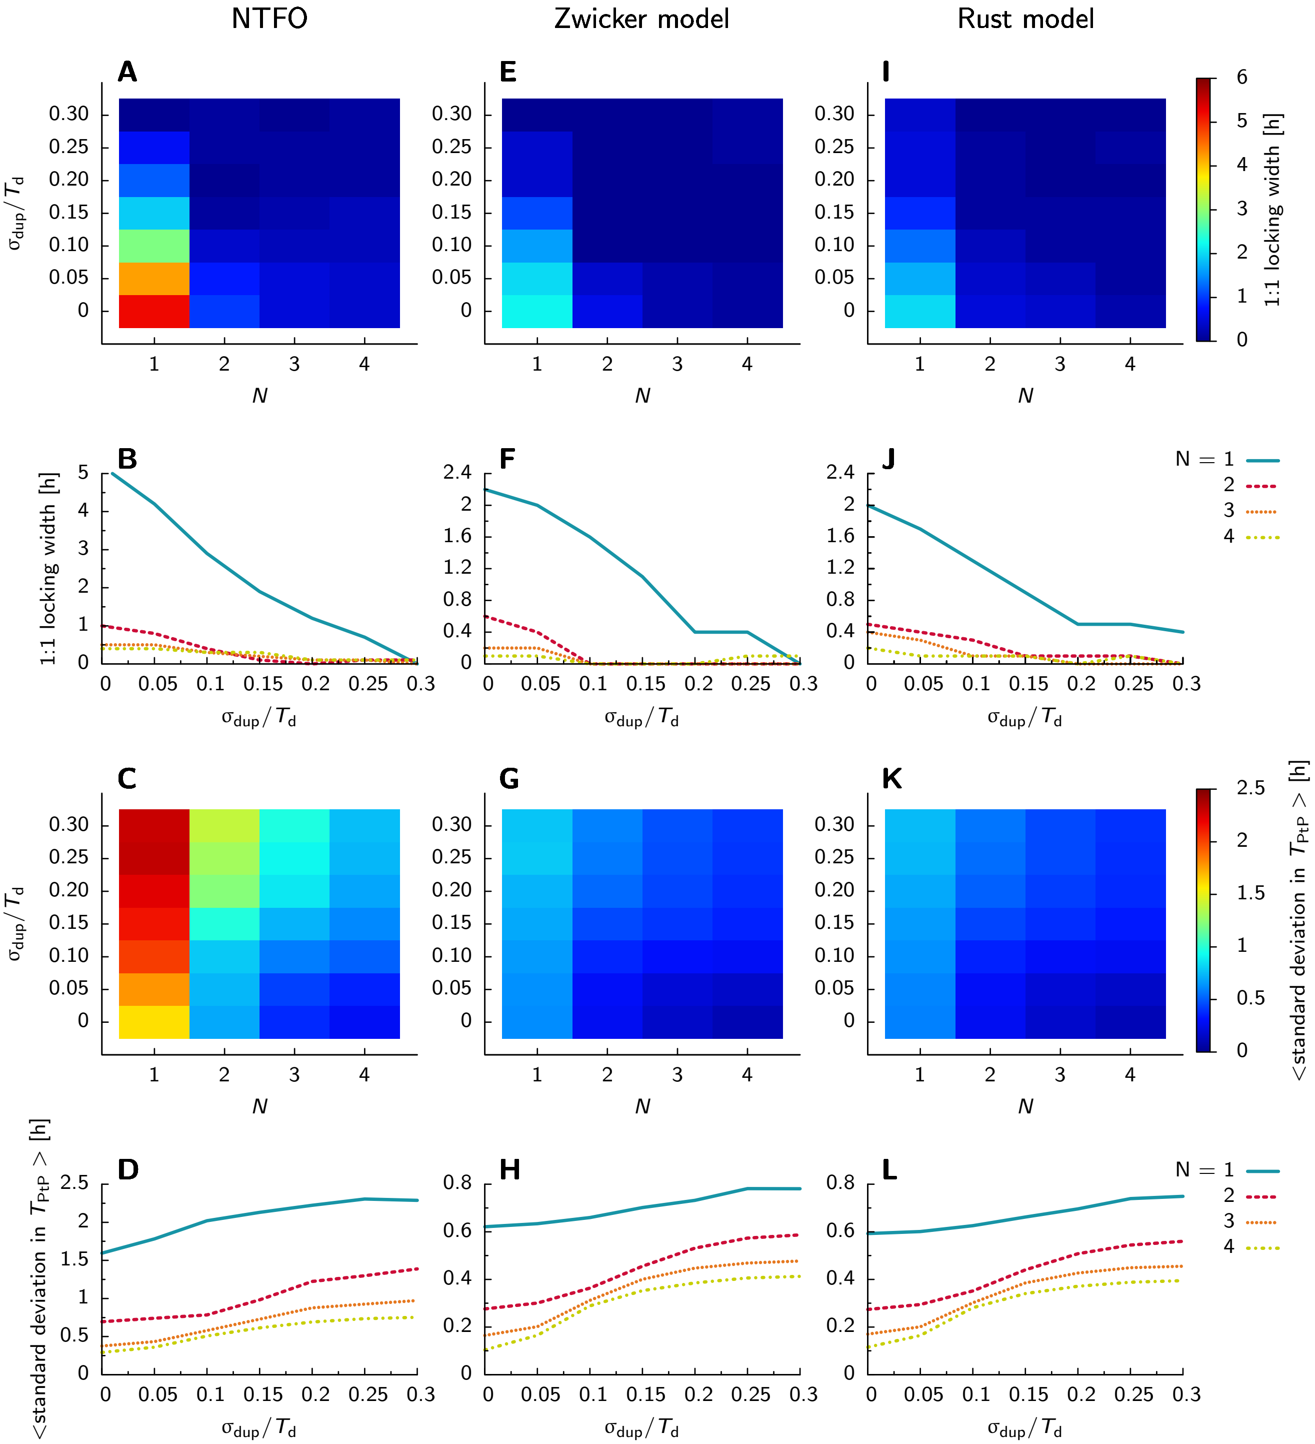


FIG. S6. Heat plots of the width of the 1:1 locking region (panels, A, E, I) and the average standard deviation of the peak-to-peak time (panels C, G, K), as a function of the initial gene copy number $N$ and the standard deviation in the gene replication time $\sigma_{\rm dup}/T_{\rm d}$, for the NTFO model (panels A–D), the Zwicker TTC-PPC model [35] (panels E–H), and the Rust TTC-PPC model [26, 35] (panel I–L). Panels B,D,F,H,J,L show the same data as in the plots immediately above them, but as a function of $\sigma_{\rm dup}/T_{\rm d}$, for different values of $N$; *note the difference in scale of the y-axes* in these panels. The average standard deviation in the peak-to-peak time is the standard deviation in the peak-to-peak time averaged over $6 < T_{\rm d} < 52$; it is a measure for the erratic behavior of the clock outside the locking regions. It is seen that in all models the width of the locking region rapidly decreases with both $N$ and $\sigma_{\rm dup}/T_{\rm d}$. However, the average standard deviation in the peak-to-peak time decreases with $N$, but increases with $\sigma_{\rm dup}/T_{\rm d}$. Clearly, while having multiple chromosome copies is a powerful strategy for preventing locking, increasing the stochasticity in the timing of gene replication is not—decreasing locking at the expense of much greater variation in the length of the periodic is unlikely to be functionally advantageous. Comparing the two models with a PPC to the NTFO model shows that adding a PPC to a TTC also decreases both the width of the locking region and the average standard deviation in the peak-to-peak time. Combining both features—a PPC and multiple chromosome copies—gives the strongest reduction in the coupling of the clock to the cell cycle.

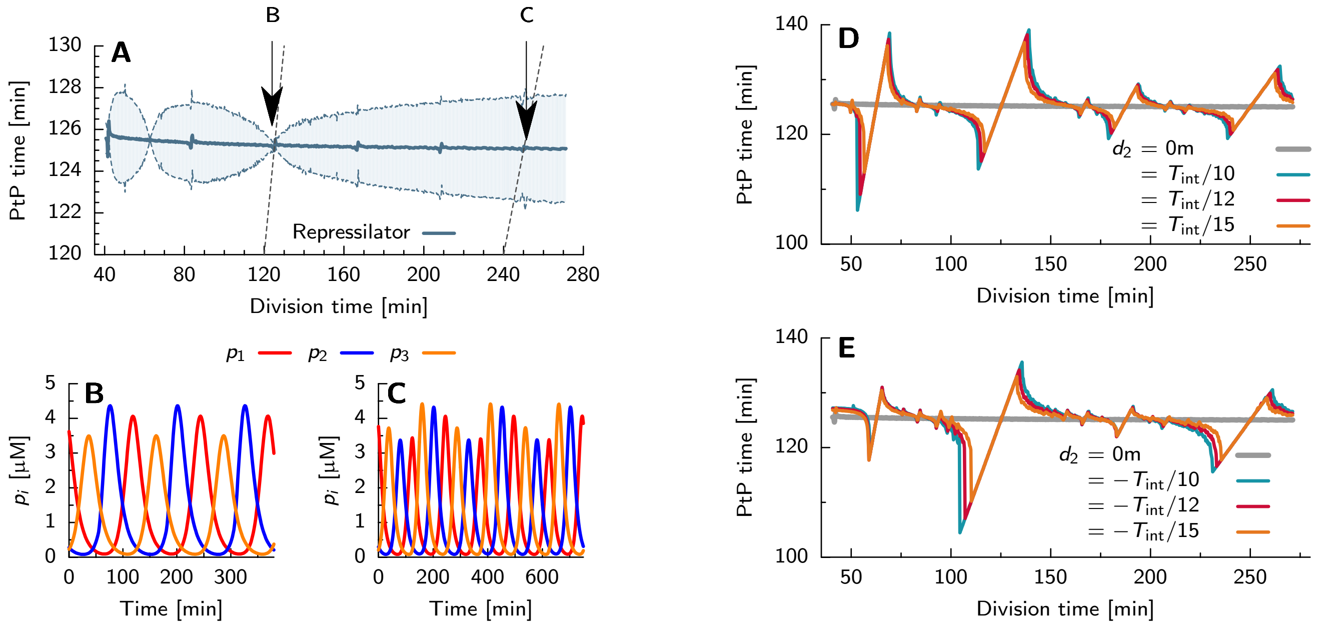


FIG. S7. The repressilator [49] can strongly lock to the cell cycle, and the strength of locking depends sensitively on the temporal order in which the respective genes are replicated during the cell cycle. (A) Average (solid line) and standard deviation (shaded region) of the peak-to-peak time $T_{\rm PtP}$ as a function of the division time $T_{\rm d}$ for a repressilator with initial gene copy number $N = 1$. The repressilator has an intrinsic period of $T_{\rm int} = 125$ minutes and the three genes are replicated simultaneously. The locking regions around $T_{\rm int}$ and $2T_{\rm int}$ are almost absent. (B and C) Representative time traces of the concentrations of the three repressilator proteins, $p_1(t)$ (red), $p_2(t)$ (blue) and $p_3(t)$ (orange), for the cell-division times indicated by the arrows in panel A. (B) When $T_{\rm d} = T_{\rm int}$, the oscillations are very regular (almost no variance in the PtP-times), but each protein concentration has a different amplitude. (C) At $T_{\rm d} = 2T_{\rm int}$, all three protein concentrations switch between a small and a large amplitude in successive oscillation cycles. Panels D and E show the effect of varying the timing of replication of the three genes. For clarity, we only show the average peak-to-peak time as a function of $T_{\rm d}$, not the standard deivation. We assume that the $p_1$ gene is always replicated halfway through the cell cycle, $d_1 = 0$, and that the $p_2$ and $p_3$ genes are replicated with delays $d_2$ and $d_3 = -d_2$, respectively. The gray line gives the situation where all genes are replicated simultaneously, $d_1 = d_2 = d_3 = 0$. Other values of $d_2$ are given in the legend, and are written as as a fraction of the intrinsic period $T_{\rm int}$ of the oscillator. Panel D shows scenarios for which $d_3 < d_1 < d_2$, meaning that the chronological order of replication is $p_3$ before $p_1$ before $p_2$. Panel E shows situations for which $d_2 < d_1 < d_3$. Remarkably, for all $d_2 = -d_3 \neq 0$, there is significant locking. For the scenarios in panel E, however, the width of the 1:1 locking region is the largest; this is because the temporal order the genes' replication during the cell cycle is the same as that of their expression in the oscillator, i.e. $p_2, p_1, p_3$ (see panels B,C). Clearly, the timing of gene replication can markedly affect locking, which means that the spatial distribution of the genes over the chromosome can be of critical importance in the interaction between the clock and the cell cycle.

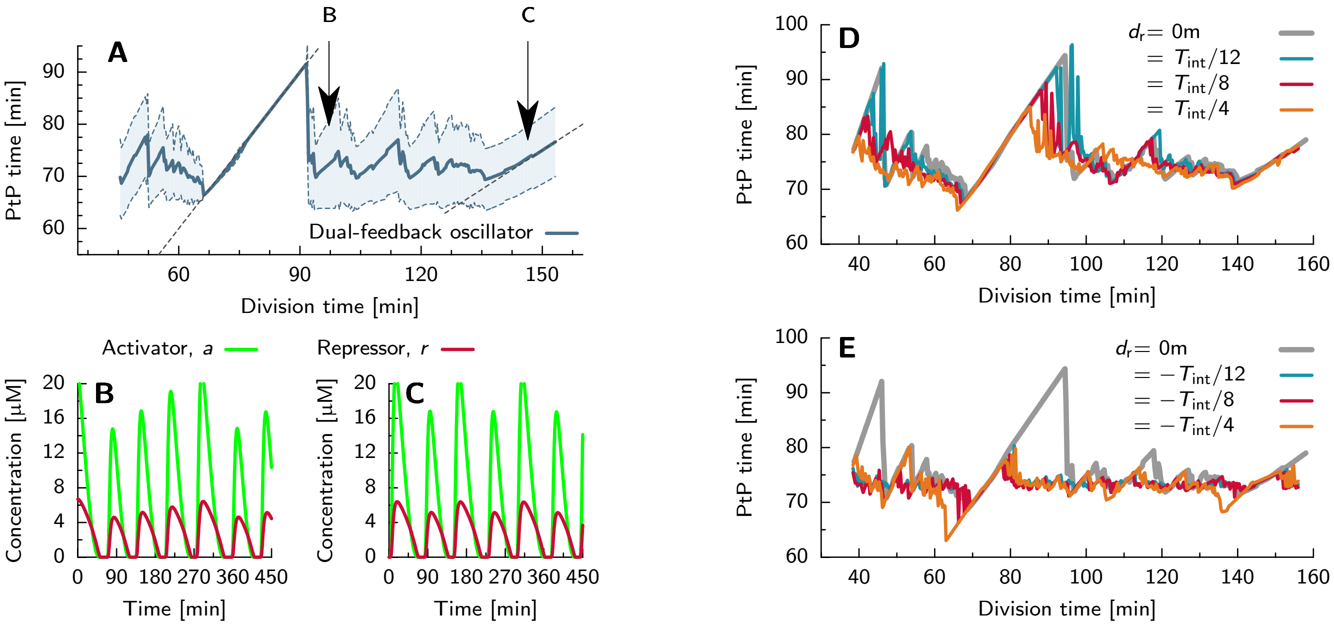


FIG. S8. The dual-feedback oscillator [50] can strongly lock to the cell cycle, and the strength of locking depends on the temporal order in which the genes are replicated during the cell cycle. The intrinsic period of the oscillator $T_{\rm int} = 73$ minutes. (A) Average (solid line) and standard deviation (shaded region) of the peak-to-peak time $T_{\rm PtP}$ as a function of the division time $T_{\rm d}$ for a dual-feedback oscillator with initial gene copy number $N = 1$ and all genes replicated simultaneously. The region of 1:1 locking (around $T_{\rm d} = 73$ min) with the cell cycle (left dashed line) has widened considerably compared to the NTFO model (compare with Fig.2 of the main text). (B and C) Representative time traces for the division times indicated by the arrows in panel A. Shown are the activator and repressor concentrations $a(t)$ (green line) and $r(t)$ (green line), respectively. At a cell-division time of $T_{\rm d} = 96$ min (B), just outside the region where the oscillator is locked to the cell cycle, the time traces show very irregular behavior resulting in a large variance in the PtP times. At $T_{\rm d} = 2T_{\rm int}$ (C), the oscillations switch between a small and a large amplitude in successive oscillation cycles, just as in the NTFO. (D and E) The effect of the order of gene replication during the cell cycle. For clarity, only the average peak-to-peak time as a function of $T_{\rm d}$ is shown, not the standard deivation. We assume that the activator gene is always replicated halfway through the cell cycle, $d_{\rm a} = 0$, and that the repressor gene is replicated with a delay $d_{\rm r}$. In both figures, the gray line gives the situation where the genes are replicated simultaneously, $d_{\rm r} = 0$. Other values of $d_{\rm r}$ are given in the legend, and are written as as a fraction of the intrinsic period $T_{\rm int}$ of the oscillator. (D) positive $d_{\rm r}$; the repressor gene is replicated after the activator gene. (E) negative $d_{\rm r}$; the repressor gene is replicated before the activator gene. Panel D shows that locking decreases as $d_{\rm r}$ becomes more positive, while panel E shows that the size of the 1:1 locking region depends non-monotonically on $d_{\rm r}$ for $d_{\rm r} < 0$. Comparing the behavior of the dual-feedback oscillator, which exhibits the strongest entrainment when the genes are replicated simulateneously, with that of the repressilator, which shows the weakest coupling when the genes are replicated together, shows that the influence of the cell cycle on the clock depends in a non-trivial way on the architecture of the clock and on the nature of the driving signal.

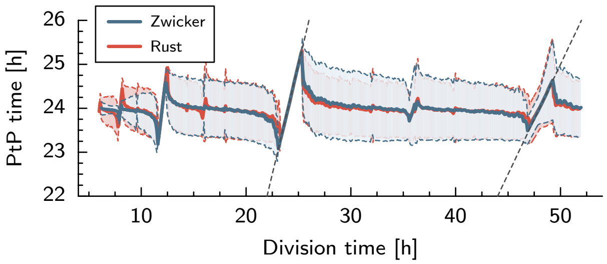


FIG. S9. A TTC combined with a PPC based on the model of Rust *et al.* [26] is susceptible to periodic gene replication. The average and standard deviation in the peak-to-peak time $T_{\rm PtP}$ for the phosphorylation fraction $p(t)$ for the Rust model and the model of Zwicker *et al.* [35]. Clearly, the two models are similarly affected by the presence of the cell cycle.
